# Supplementary material for: Nontrivial Quantum Cellular Automata in Higher Dimensions
Source: arXiv:1812.01625 source file (2022-04-21)
Supplement: Supplementary file 1 [file Supp-Mathematica.pdf]

# Tools

## Variables of Laurent polynomial ring:

```
In[1]:= Protect[x, y, z];

In[2]:= translationVariables = {x, y, z};
```

## antipode(f): an involutive automorphism of Laurent polynomial ring

## dagger = antipode followed by transpose

## symprod[v, w] = symplectic product = dagger[v].λ.w

```
In[3]:= monomialAntipode[f_] :=
         Module[{e, v, c, mono},
          v = Intersection[Variables[f], translationVariables];
          e = Map[Exponent[f, #] &, v];
          mono = Apply[Times, Power[v, e]];
          c = If[mono === 1, f, Coefficient[f, mono]];
          c * Apply[Times, Power[v, -e]]]
        antipode[f_] :=
         Module[{ff, fff},
          ff = Expand[f];
          If[Head[ff] === Plus, fff = ff, fff = {ff}];
          Apply[Plus, Map[monomialAntipode, Apply[List, Expand[fff]]]]
         ]

In[5]:= dagger[m_] := If[ArrayDepth[m] == 2,
          Transpose[Map[antipode, m, {ArrayDepth[m]}]], Map[antipode, m, {ArrayDepth[m]}]]

In[6]:= symplecticMatrix[n_] := KroneckerProduct[{{0, 1}, {-1, 0}}, IdentityMatrix[n]]
        symprod[v_, w_] := Expand[dagger[v].symplecticMatrix[Length[w] / 2].w]
```

## Everything modulo 2

```
In[8]:= pmod2[x_] := PolynomialMod[x, 2]
```

### Extracting the constant term of a Laurent polynomial: coe( Laurent poly ) = its constant term.

In[9]:=
```
monomialTest[f_] :=
 Module[{e, v, c, mono},
  v = Intersection[Variables[f], translationVariables];
  If[v == {}, f, 0]
 ]
coe[f_] :=
 Module[{ff, fff},
  ff = Expand[f];
  If[Head[ff] === Plus, fff = ff, fff = {ff}];
  Apply[Plus, Map[monomialTest, Apply[List, Expand[fff]]]]
 ]
```

### Counting the number of Y components modulo 2

In[11]:=
```
realV[v_] := coe@pmod2[
   dagger[v[[ ;; Length[v] / 2]]].v[[Length[v] / 2 + 1 ;;]]
  ](* This is for a vector of Laurent polynomials. *)
```

In[12]:=
```
realQ[Q_] := Table[realV[Q[[ ;; , k]]], {k, 1, Dimensions[Q][[2]]}]
(* This is for a matrix of Laurent polynomials,
where each column represents a Pauli operator. *)
```

# Walker-Wang Model with three-fermion surface

In[13]:=

$$\text{sigma} = \begin{pmatrix}
1+x^{-1} & 0 & 0 & 0 & x^{-1}+yz & 0 & 0 & yz \\
1+y^{-1} & 0 & 0 & y^{-1}+xz & 0 & 0 & xz & 0 \\
1+z^{-1} & 0 & z^{-1}+xy & 0 & 0 & xy & 0 & 0 \\
0 & 1+x^{-1} & 0 & 0 & x^{-1} & 0 & 0 & x^{-1}+yz \\
0 & 1+y^{-1} & 0 & y^{-1} & 0 & 0 & y^{-1}+xz & 0 \\
0 & 1+z^{-1} & z^{-1} & 0 & 0 & z^{-1}+xy & 0 & 0 \\
0 & 0 & 1+y & 1+z & 0 & 0 & 0 & 0 \\
0 & 0 & 1+x & 0 & 1+z & 0 & 0 & 0 \\
0 & 0 & 0 & 1+x & 1+y & 0 & 0 & 0 \\
0 & 0 & 0 & 0 & 0 & 1+y & 1+z & 0 \\
0 & 0 & 0 & 0 & 0 & 1+x & 0 & 1+z \\
0 & 0 & 0 & 0 & 0 & 0 & 1+x & 1+y
\end{pmatrix};$$

In[14]:=
```
symprod[sigma, sigma] // pmod2
```

Out[14]=
```
{{0, 0, 0, 0, 0, 0, 0, 0}, {0, 0, 0, 0, 0, 0, 0, 0},
 {0, 0, 0, 0, 0, 0, 0, 0}, {0, 0, 0, 0, 0, 0, 0, 0}, {0, 0, 0, 0, 0, 0, 0, 0},
 {0, 0, 0, 0, 0, 0, 0, 0}, {0, 0, 0, 0, 0, 0, 0, 0}, {0, 0, 0, 0, 0, 0, 0, 0}}
```

Here, symprod being zero implies that the Hamiltonian consists of commuting terms.

# Rearrangement of Hamiltonian terms: a different generating set for the group generated by the Hamiltonian terms

In[15]:= columnOperation =

$$\left\{\left\{xy+\frac{1}{xyz^2}+\frac{1}{z},\ 1+xyz,\ 0,\ 0,\ 0,\ 1,\ z+xyz^2,\ yz+xy^2z^2\right\},\ \{0,1,0,0,0,0,0,0\},\right.$$
$$\left\{1+\frac{1}{xyz^2}+\frac{1}{z}+\frac{1}{xyz},\ 1+z,\ 1,\ 0,\ 0,\ \frac{1}{xy},\ \frac{1}{xy}+z+\frac{z}{xy}+z^2,\ \frac{1}{x}+\frac{z}{x}+yz+yz^2\right\},$$
$$\left\{\frac{1}{xz^2}+\frac{1}{xyz^2}+\frac{1}{z}+\frac{y}{z},\ 1+y,\ 0,\ 1,\ 0,\ \frac{1}{xz}+\frac{1}{xyz},\ \frac{1}{x}+\frac{1}{xy}+\frac{1}{xyz}+z+yz,\ \frac{1}{x}+\frac{y}{x}+yz+y^2z\right\},$$
$$\left\{\frac{1}{yz^2}+\frac{1}{xyz^2}+\frac{1}{z}+\frac{x}{z},\ 1+x,\ 0,\ 0,\ 1,\ \frac{1}{yz}+\frac{1}{xyz},\ \frac{1}{y}+\frac{1}{xy}+z+xz,\ 1+\frac{1}{x}+\frac{1}{xyz}+yz+xyz\right\},$$
$$\left\{\frac{1}{xyz^2}+\frac{1}{xyz},\ 0,0,0,0,1,0,0\right\},\ \left\{\frac{1}{xz^2}+\frac{1}{xyz^2},\ 0,0,0,0,0,1,0\right\},$$
$$\left.\left\{\frac{1}{yz^2}+\frac{1}{xyz^2},\ 0,0,0,0,0,0,1\right\}\right\};$$

In[16]:= Dimensions[columnOperation]

Out[16]= {8, 8}

In[17]:= Det[columnOperation] // pmod2

Out[17]= 1

The columnOperation is invertible, and therefore the old set and the new set of terms generate the same stabilizer group.

In[18]:= newsigma = sigma.columnOperation // pmod2 // Expand;
newsigma // MatrixForm

Out[19]//MatrixForm=

$$\begin{pmatrix}
0 & 0 & 0 & 0 & \frac{1}{x}+yz & \frac{1}{x^2yz}+\frac{1}{xyz} & \frac{1}{x^2y}+\frac{1}{xy}+z+\frac{z}{x} & \frac{1}{x^2}+\frac{1}{x^2yz}+\frac{yz}{x} \\
0 & 0 & 0 & \frac{1}{y}+xz & 0 & \frac{1}{xy^2z}+\frac{1}{xyz} & \frac{1}{xy^2}+\frac{1}{y}+\frac{1}{xy}+\frac{1}{xy^2z}+z+xz+\frac{z}{y} & \frac{1}{x}+\frac{1}{xy}+z+yz \\
0 & 0 & xy+\frac{1}{z} & 0 & 0 & xy+\frac{1}{z}+\frac{1}{xyz} & 1+\frac{1}{xy}+\frac{1}{xyz}+z & \frac{1}{x}+y+\frac{1}{xz}+yz \\
0 & 0 & 0 & 0 & \frac{1}{x} & \frac{1}{x^2yz}+\frac{1}{xyz} & \frac{1}{x^2y}+\frac{1}{xy}+z+\frac{z}{x} & \frac{1}{x^2}+\frac{1}{x^2yz}+\frac{yz}{x} \\
0 & 0 & 0 & \frac{1}{y} & 0 & \frac{1}{xy^2z}+\frac{1}{xyz} & \frac{1}{xy^2}+\frac{1}{y}+\frac{1}{xy}+\frac{1}{xy^2z}+z+xz+\frac{z}{y} & \frac{1}{x}+\frac{1}{xy}+z+yz \\
0 & 0 & \frac{1}{z} & 0 & 0 & xy+\frac{1}{z}+\frac{1}{xyz} & 1+\frac{1}{xy}+\frac{1}{xyz}+z & \frac{1}{x}+y+\frac{1}{xz}+yz \\
0 & 0 & 1+y & 1+z & 0 & \frac{1}{xz}+\frac{1}{xyz} & \frac{1}{xy}+\frac{1}{xyz} & 0 \\
0 & 0 & 1+x & 0 & 1+z & \frac{1}{yz}+\frac{1}{xyz} & 0 & \frac{1}{xy}+\frac{1}{xyz} \\
0 & 0 & 0 & 1+x & 1+y & 0 & \frac{1}{yz}+\frac{1}{xyz} & \frac{1}{xz}+\frac{1}{xyz} \\
0 & 0 & 0 & 0 & 0 & 1+y & 1+z & 0 \\
0 & 0 & 0 & 0 & 0 & 1+x & 0 & 1+z \\
0 & 0 & 0 & 0 & 0 & 0 & 1+x & 1+y
\end{pmatrix}$$

The first two columns being zero in this 12-by-8 matrix means that the stabilizer group is generated by six terms and their translates, in contrast to eight terms in the original Hamiltonian. The six nonzero columns constitute the polynomial representation of a separator.

### Reality: Time-reversal invariance

In[20]:=
```
realQ[newsigma]
```

Out[20]=
```
{0, 0, 0, 0, 0, 0, 0, 0}
```

Every element of the separator contains an even number of tensor component Y. Therefore, in the basis where X and Z are real matrices, the separator is also real.

---

# Clifford QCA

In[21]:=

$$\text{theQCA} = \left\{\left\{\frac{1}{y\,z}, 0, 0, \frac{1}{y\,z}, 0, 0, 0, 0, 0, 0, 0, 0\right\}, \left\{0, \frac{1}{x\,z}, 0, 0, \frac{1}{x\,z}, 0, 0, 0, 0, 0, 0, 0\right\},\right.$$

$$\left\{0, 0, z^2, 0, 0, z^2, 0, 0, 0, 0, 0, 0\right\}, \left\{x\,y + x\,y^2 + \frac{1}{z} + \frac{y}{z} + x\,z + x\,y\,z,\right.$$

$$y + \frac{1}{x\,z} + \frac{y}{x\,z} + x\,y^2\,z + x^2\,y^3\,z^2 + y\,z^3 + x\,y\,z^3 + y^2\,z^3 + x^3\,y^4\,z^3 + y\,z^4 + x\,y\,z^4 + y^2\,z^4 + x\,y^2\,z^4 +$$

$$x^3\,y^2\,z^4 + x^2\,y^3\,z^4 + x\,y^4\,z^4 + x^4\,y^5\,z^4 + y\,z^5 + x\,y\,z^5 + y^2\,z^5 + x\,y^2\,z^5 + x^3\,y^2\,z^5 + x^4\,y^3\,z^5 + x\,y^4\,z^5 +$$

$$x^3\,y^4\,z^5 + x^2\,y^5\,z^5 + x^4\,y^5\,z^5 + x^5\,y^5\,z^5 + x^4\,y^6\,z^5 + x^5\,y^6\,z^5 + x^2\,y^3\,z^6 + x^3\,y^3\,z^6 + x^4\,y^3\,z^6 +$$

$$x^2\,y^4\,z^6 + x^3\,y^4\,z^6 + x^2\,y^5\,z^6 + x^5\,y^5\,z^6 + x^4\,y^6\,z^6 + x^5\,y^6\,z^6 + x^2\,y^3\,z^7 + x^3\,y^3\,z^7 + x^2\,y^4\,z^7 + x^3\,y^4\,z^7,$$

$$1 + y + \frac{1}{x\,z} + \frac{1}{x\,y\,z} + y\,z + x\,y\,z + y^2\,z + x\,y^2\,z + z^2 + x\,z^2 + x\,y\,z^2 + y^2\,z^2 + z^3 + x\,z^3 + x\,y\,z^3 +$$

$$y^2\,z^3 + x^2\,y^2\,z^3 + x^2\,y^3\,z^3 + x^2\,y^2\,z^4 + x^2\,y^3\,z^4 + x^3\,y^3\,z^4 + x^3\,y^4\,z^4 + z^5 + x\,z^5 + x^3\,y\,z^5 + y^2\,z^5 +$$

$$x\,y^2\,z^5 + x^3\,y^2\,z^5 + x\,y^3\,z^5 + x^3\,y^3\,z^5 + x\,y^4\,z^5 + x^3\,y^4\,z^5 + x^4\,y^4\,z^5 + x^4\,y^5\,z^5 + x^4\,y^2\,z^6 + x^4\,y^3\,z^6 +$$

$$x^2\,y^4\,z^6 + x^5\,y^4\,z^6 + x^2\,y^5\,z^6 + x^4\,y^5\,z^6 + x^4\,y^6\,z^6 + x^5\,y^6\,z^6 + x^2\,y^2\,z^7 + x^3\,y^2\,z^7 + x^2\,y^4\,z^7 + x^3\,y^4\,z^7,$$

$$1 + \frac{1}{y}, y + \frac{1}{x\,z} + \frac{y}{x\,z} + x\,y^2\,z + z^2 + \frac{z^2}{x} + \frac{y\,z^2}{x} + x^2\,y^3\,z^2 + z^3 + \frac{z^3}{x} + y\,z^3 + \frac{y\,z^3}{x} + x^2\,y\,z^3 +$$

$$x\,y^2\,z^3 + y^3\,z^3 + x^3\,y^4\,z^3 + z^4 + \frac{z^4}{x} + y\,z^4 + \frac{y\,z^4}{x} + x^2\,y\,z^4 + x^3\,y^2\,z^4 + y^3\,z^4 + x^2\,y^3\,z^4 +$$

$$x\,y^4\,z^4 + x^3\,y^4\,z^4 + x^4\,y^4\,z^4 + x^3\,y^5\,z^4 + x^4\,y^5\,z^4 + x\,y^2\,z^5 + x^2\,y^2\,z^5 + x^3\,y^2\,z^5 + x\,y^3\,z^5 +$$

$$x^2\,y^3\,z^5 + x\,y^4\,z^5 + x^4\,y^4\,z^5 + x^3\,y^5\,z^5 + x^4\,y^5\,z^5 + x\,y^2\,z^6 + x^2\,y^2\,z^6 + x\,y^3\,z^6 + x^2\,y^3\,z^6,$$

$$1 + \frac{1}{x} + y + \frac{y}{x} + \frac{1}{x\,z} + \frac{1}{x\,y\,z} + z + \frac{z}{y} + \frac{z}{x\,y} + \frac{y\,z}{x} + z^2 + \frac{z^2}{y} + \frac{z^2}{x\,y} + \frac{y\,z^2}{x} + x\,y\,z^2 + x\,y^2\,z^2 +$$

$$x\,y\,z^3 + x\,y^2\,z^3 + x^2\,y^2\,z^3 + x^2\,y^3\,z^3 + x^2\,z^4 + \frac{z^4}{y} + \frac{z^4}{x\,y} + y\,z^4 + \frac{y\,z^4}{x} + x^2\,y\,z^4 +$$

$$y^2\,z^4 + x^2\,y^2\,z^4 + y^3\,z^4 + x^2\,y^3\,z^4 + x^3\,y^3\,z^4 + x^3\,y^4\,z^4 + x^3\,y\,z^5 + x^3\,y^2\,z^5 + x\,y^3\,z^5 +$$

$$x^4\,y^3\,z^5 + x\,y^4\,z^5 + x^3\,y^4\,z^5 + x^3\,y^5\,z^5 + x^4\,y^5\,z^5 + x\,y\,z^6 + x^2\,y\,z^6 + x\,y^3\,z^6 + x^2\,y^3\,z^6,$$

$$1 + \frac{1}{y} + \frac{x}{y} + x^2\,y + x\,y^2 + x^2\,y^2 + \frac{1}{z} + \frac{x}{z} + \frac{y}{z} + \frac{x\,y}{z} + z + x\,z + x^2\,z + \frac{z}{y} + \frac{x\,z}{y} + x\,y^2\,z + x^2\,y^2\,z +$$

$$x\,z^2 + x^2\,z^2 + x\,y^2\,z^2 + z^3 + x\,z^3 + x^3\,z^3 + \frac{z^3}{y} + \frac{x\,z^3}{y} + x\,y\,z^3 + x^2\,y\,z^3 + x^3\,y^3\,z^3 + x\,z^4 + x^2\,z^4 +$$

$$x\,y\,z^4 + x^2\,y\,z^4 + x^3\,y^3\,z^4 + x^4\,y^3\,z^4 + x^5\,y^3\,z^4 + x\,y\,z^5 + x^3\,y\,z^5 + x\,y^2\,z^5 + x^3\,y^2\,z^5 + x^4\,y^2\,z^5 +$$

$$x^5 y^2 z^5 + x^2 y^4 z^5 + x^3 y^4 z^5 + x^4 y^4 z^5 + x^6 y^4 z^5 + x^6 y^5 z^5 + x^3 y^2 z^6 + x^4 y^2 z^6 + x^3 y^3 z^6 +$$
$$x^4 y^3 z^6 + x^5 y^3 z^6 + x^3 y^5 z^6 + x^6 y^5 z^6 + x^5 y^6 z^6 + x^6 y^6 z^6 + x^3 y^3 z^7 + x^4 y^3 z^7 + x^3 y^4 z^7 + x^4 y^4 z^7,$$

$$1 + \frac{1}{y} + \frac{1}{x y} + y + \frac{y}{x} + x y + y^2 + x y^3 + \frac{1}{z} + \frac{1}{x z} + \frac{y}{x z} + \frac{y^2}{z} + x z + \frac{z}{y} + \frac{z}{x y} + \frac{y z}{x} + x y z + y^2 z + z^2 + x z^2 +$$
$$y^2 z^2 + x y^2 z^2 + x^2 z^3 + \frac{z^3}{y} + \frac{z^3}{x y} + y z^3 + \frac{y z^3}{x} + x^2 y z^3 + y^2 z^3 + y^3 z^3 + z^4 + x z^4 + y^2 z^4 + x y^2 z^4 +$$
$$x^3 y^3 z^4 + x^4 y^3 z^4 + x^4 y^4 z^4 + x^3 y^5 z^4 + x y z^5 + x^2 y z^5 + x^4 y^2 z^5 + x y^3 z^5 + x^2 y^3 z^5 + x^4 y^3 z^5 +$$
$$x^2 y^4 z^5 + x^5 y^4 z^5 + x^2 y^5 z^5 + x^4 y^5 z^5 + x^4 y^6 z^5 + x^5 y^6 z^5 + x^2 y^2 z^6 + x^3 y^2 z^6 + x^2 y^4 z^6 + x^3 y^4 z^6,$$

$$1 + \frac{1}{y} + x y + x y^2 + \frac{1}{z} + \frac{y}{z} + x z + x y z + \frac{z^2}{x} + \frac{z^2}{y} + \frac{z^2}{x y} + \frac{z^3}{x} + x z^3 + x^2 z^3 + \frac{z^3}{y} + \frac{z^3}{x y} + y z^3 +$$
$$x y z^3 + y^2 z^3 + \frac{z^4}{x} + x z^4 + x^2 z^4 + \frac{z^4}{y} + \frac{z^4}{x y} + y z^4 + x y z^4 + y^2 z^4 + x^3 y^3 z^4 + x^4 y^3 z^4 +$$
$$x^3 y^4 z^4 + z^5 + x z^5 + y z^5 + x^2 y z^5 + x y^2 z^5 + x^2 y^2 z^5 + x^4 y^2 z^5 + x^3 y^3 z^5 + x^4 y^3 z^5 + x^2 y^4 z^5 +$$
$$x^3 y^4 z^5 + x^5 y^4 z^5 + x^4 y^5 z^5 + x^5 y^5 z^5 + x y z^6 + x^2 y z^6 + x y^2 z^6 + x^3 y^2 z^6 + x^4 y^2 z^6 + x^2 y^3 z^6 +$$
$$x^3 y^3 z^6 + x^2 y^4 z^6 + x^5 y^4 z^6 + x^4 y^5 z^6 + x^5 y^5 z^6 + x^2 y^2 z^7 + x^3 y^2 z^7 + x^2 y^3 z^7 + x^3 y^3 z^7,$$

$$1 + \frac{1}{y} + \frac{x}{y} + x^2 y + x y^2 + x^2 y^2 + \frac{1}{z} + \frac{x}{z} + \frac{y}{z} + \frac{x y}{z} + z + x z + x^2 z + \frac{z}{y} + \frac{x z}{y} + x y^2 z + x^2 y^2 z +$$
$$x z^2 + x^2 z^2 + x y^2 z^2 + z^3 + x z^3 + x^3 z^3 + \frac{z^3}{y} + \frac{x z^3}{y} + x y z^3 + x^2 y z^3 + x^3 y^3 z^3 + x z^4 + x^2 z^4 +$$
$$x y z^4 + x^2 y z^4 + x^3 y^3 z^4 + x^4 y^3 z^4 + x^5 y^3 z^4 + x y z^5 + x^3 y z^5 + x y^2 z^5 + x^3 y^2 z^5 + x^4 y^2 z^5 +$$
$$x^5 y^2 z^5 + x^2 y^4 z^5 + x^3 y^4 z^5 + x^4 y^4 z^5 + x^6 y^4 z^5 + x^6 y^5 z^5 + x^3 y^2 z^6 + x^4 y^2 z^6 + x^3 y^3 z^6 +$$
$$x^4 y^3 z^6 + x^5 y^3 z^6 + x^3 y^5 z^6 + x^6 y^5 z^6 + x^5 y^6 z^6 + x^6 y^6 z^6 + x^3 y^3 z^7 + x^4 y^3 z^7 + x^3 y^4 z^7 + x^4 y^4 z^7,$$

$$1 + \frac{1}{y} + \frac{1}{x y} + y + \frac{y}{x} + x y + y^2 + x y^3 + \frac{1}{z} + \frac{1}{x z} + \frac{y}{x z} + \frac{y^2}{z} + x z + \frac{z}{y} + \frac{z}{x y} + \frac{y z}{x} + x y z + y^2 z + z^2 + x z^2 +$$
$$y^2 z^2 + x y^2 z^2 + x^2 z^3 + \frac{z^3}{y} + \frac{z^3}{x y} + y z^3 + \frac{y z^3}{x} + x^2 y z^3 + y^2 z^3 + y^3 z^3 + z^4 + x z^4 + y^2 z^4 + x y^2 z^4 +$$
$$x^3 y^3 z^4 + x^4 y^3 z^4 + x^4 y^4 z^4 + x^3 y^5 z^4 + x y z^5 + x^2 y z^5 + x^4 y^2 z^5 + x y^3 z^5 + x^2 y^3 z^5 + x^4 y^3 z^5 +$$
$$x^2 y^4 z^5 + x^5 y^4 z^5 + x^2 y^5 z^5 + x^4 y^5 z^5 + x^4 y^6 z^5 + x^5 y^6 z^5 + x^2 y^2 z^6 + x^3 y^2 z^6 + x^2 y^4 z^6 + x^3 y^4 z^6,$$

$$1 + \frac{1}{y} + x y + x y^2 + \frac{1}{z} + \frac{y}{z} + x z + x y z + \frac{z^2}{x} + \frac{z^2}{y} + \frac{z^2}{x y} + \frac{z^3}{x} + x z^3 + x^2 z^3 + \frac{z^3}{y} + \frac{z^3}{x y} + y z^3 +$$
$$x y z^3 + y^2 z^3 + \frac{z^4}{x} + x z^4 + x^2 z^4 + \frac{z^4}{y} + \frac{z^4}{x y} + y z^4 + x y z^4 + y^2 z^4 + x^3 y^3 z^4 + x^4 y^3 z^4 +$$
$$x^3 y^4 z^4 + z^5 + x z^5 + y z^5 + x^2 y z^5 + x y^2 z^5 + x^2 y^2 z^5 + x^4 y^2 z^5 + x^3 y^3 z^5 + x^4 y^3 z^5 + x^2 y^4 z^5 +$$
$$x^3 y^4 z^5 + x^5 y^4 z^5 + x^4 y^5 z^5 + x^5 y^5 z^5 + x y z^6 + x^2 y z^6 + x y^2 z^6 + x^3 y^2 z^6 + x^4 y^2 z^6 + x^2 y^3 z^6 +$$
$$x^3 y^3 z^6 + x^2 y^4 z^6 + x^5 y^4 z^6 + x^4 y^5 z^6 + x^5 y^5 z^6 + x^2 y^2 z^7 + x^3 y^2 z^7 + x^2 y^3 z^7 + x^3 y^3 z^7 \},$$

$$\{ \frac{1}{y^2 z^6} + \frac{1}{x y^2 z^6} + \frac{1}{y z^6} + \frac{1}{x y z^6} + \frac{1}{x^3 y^4 z^5} + \frac{1}{x^2 y^4 z^5} + \frac{1}{y^3 z^5} + \frac{1}{x^3 y^3 z^5} + \frac{1}{y^2 z^5} +$$
$$\frac{1}{x y^2 z^5} + \frac{1}{y z^5} + \frac{1}{x^2 y z^5} + \frac{1}{x y z^5} + \frac{1}{x z^4} + \frac{x}{z^4} + \frac{x^2}{z^4} + \frac{1}{x^3 y^4 z^4} + \frac{1}{x^2 y^4 z^4} + \frac{1}{y^3 z^4} +$$
$$\frac{1}{x^3 y^3 z^4} + \frac{1}{x^2 y^3 z^4} + \frac{1}{x y^2 z^4} + \frac{x}{y^2 z^4} + \frac{1}{x^2 y z^4} + \frac{x y}{z^4} + \frac{x^2 y}{z^4} + \frac{1}{x z^3} + \frac{x}{z^3} + \frac{x^2}{z^3} +$$
$$\frac{1}{x^2 y^3 z^3} + \frac{x}{y^2 z^3} + \frac{1}{y z^3} + \frac{x y}{z^3} + \frac{x^2 y}{z^3} + \frac{x^2}{z^2} + \frac{1}{x y^2 z^2} + \frac{x y}{z^2} + \frac{x^2 y}{z^2} + \frac{1}{z} + \frac{x}{z} + \frac{1}{y z},$$

$$x y + x^2 y + \frac{1}{z} + \frac{1}{x z} + y z + x y z, \; 1 + x^2 + y + x^2 y + \frac{1}{y^2 z^5} + \frac{1}{x^2 y^2 z^5} + \frac{1}{y z^5} + \frac{1}{x^2 y z^5} +$$

$$\frac{1}{x^4 y^4 z^4}+\frac{1}{x^2 y^4 z^4}+\frac{1}{y^3 z^4}+\frac{1}{x^4 y^3 z^4}+\frac{1}{x^3 y^3 z^4}+\frac{1}{x y^3 z^4}+\frac{1}{x^3 y z^4}+\frac{1}{x^2 y z^4}+\frac{1}{z^3}+$$

$$\frac{1}{x^2 z^3}+\frac{1}{x z^3}+\frac{x^2}{z^3}+\frac{1}{x^3 y^3 z^3}+\frac{1}{x^2 y^3 z^3}+\frac{1}{y^2 z^3}+\frac{1}{x^2 y^2 z^3}+\frac{1}{x y^2 z^3}+\frac{x}{y^2 z^3}+\frac{y}{z^3}+$$

$$\frac{x^2 y}{z^3}+\frac{1}{x^2 y^2 z^2}+\frac{1}{x y^2 z^2}+\frac{1}{y z^2}+\frac{1}{x y z^2}+\frac{x}{z}+\frac{x^2}{z}+\frac{y}{z}+\frac{x^2 y}{z}+z+x z+y z+x y z,$$

$$\frac{1}{x^2 y^3 z^7}+\frac{1}{x y^3 z^7}+\frac{1}{x^2 y^2 z^7}+\frac{1}{x y^2 z^7}+\frac{1}{x^4 y^5 z^6}+\frac{1}{x^3 y^5 z^6}+\frac{1}{x^4 y^4 z^6}+\frac{1}{x y^4 z^6}+\frac{1}{x^2 y^3 z^6}+$$

$$\frac{1}{x y^3 z^6}+\frac{1}{x^3 y^2 z^6}+\frac{1}{x^2 y^2 z^6}+\frac{1}{x y^2 z^6}+\frac{1}{z^5}+\frac{x}{z^5}+\frac{1}{x^4 y^5 z^5}+\frac{1}{x^3 y^5 z^5}+\frac{1}{x^4 y^4 z^5}+\frac{1}{x^3 y^4 z^5}+$$

$$\frac{1}{x y^4 z^5}+\frac{1}{y^3 z^5}+\frac{1}{x^2 y^3 z^5}+\frac{1}{x^3 y^2 z^5}+\frac{1}{y z^5}+\frac{1}{x^2 y z^5}+\frac{x}{y z^5}+\frac{1}{z^4}+\frac{x}{z^4}+\frac{1}{x^3 y^4 z^4}+\frac{1}{y^3 z^4}+\frac{1}{x y^2 z^4}+$$

$$\frac{1}{y z^4}+\frac{1}{x^2 y z^4}+\frac{x}{y z^4}+\frac{1}{z^3}+\frac{x}{z^3}+\frac{1}{x^2 y^3 z^3}+\frac{x}{y z^3}+\frac{1}{x y^2 z^2}+\frac{1}{z}+\frac{x}{z}+\frac{1}{y z},\ 1+\frac{1}{x}+\frac{1}{x z}+\frac{x}{z},$$

$$1+\frac{1}{x}+\frac{1}{y}+\frac{1}{x y}+\frac{1}{x^3 y^3 z^6}+\frac{1}{x y^3 z^6}+\frac{1}{x^3 y^2 z^6}+\frac{1}{x y^2 z^6}+\frac{1}{x^5 y^5 z^5}+\frac{1}{x^3 y^5 z^5}+\frac{1}{x^5 y^4 z^5}+$$

$$\frac{1}{x^4 y^4 z^5}+\frac{1}{x^2 y^4 z^5}+\frac{1}{x y^4 z^5}+\frac{1}{x^4 y^2 z^5}+\frac{1}{x^3 y^2 z^5}+\frac{1}{x z^4}+\frac{x}{z^4}+\frac{1}{x^4 y^4 z^4}+\frac{1}{x^3 y^4 z^4}+\frac{1}{y^3 z^4}+$$

$$\frac{1}{x^3 y^3 z^4}+\frac{1}{x^2 y^3 z^4}+\frac{1}{x y^3 z^4}+\frac{1}{x^3 y z^4}+\frac{1}{x^2 y z^4}+\frac{1}{x y z^4}+\frac{x}{y z^4}+\frac{1}{x^3 y^3 z^3}+\frac{1}{x^2 y^3 z^3}+$$

$$\frac{1}{x^2 y^2 z^3}+\frac{1}{x y^2 z^3}+\frac{1}{x z^2}+\frac{x}{z^2}+\frac{1}{x^2 y^2 z^2}+\frac{1}{x y^2 z^2}+\frac{1}{y z^2}+\frac{x}{y z^2}+\frac{1}{x z}+\frac{x}{z}+\frac{1}{x y z}+\frac{x}{y z},$$

$$x+x^2+x y+x^3 y+\frac{1}{y^3 z^7}+\frac{1}{x^2 y^3 z^7}+\frac{1}{y^2 z^7}+\frac{1}{x^2 y^2 z^7}+\frac{1}{x^4 y^5 z^6}+\frac{1}{x^2 y^5 z^6}+\frac{1}{y^4 z^6}+$$

$$\frac{1}{x^4 y^4 z^6}+\frac{1}{x^3 y^4 z^6}+\frac{1}{x y^4 z^6}+\frac{1}{x^3 y^2 z^6}+\frac{1}{x^2 y^2 z^6}+\frac{1}{x y^2 z^6}+\frac{x}{y^2 z^6}+\frac{1}{x y z^6}+$$

$$\frac{x}{y z^6}+\frac{1}{z^5}+\frac{x^2}{z^5}+\frac{1}{x^2 y^4 z^5}+\frac{1}{x y^4 z^5}+\frac{1}{x^3 y^3 z^5}+\frac{1}{x y^3 z^5}+\frac{1}{y z^5}+\frac{x^2}{y z^5}+\frac{1}{z^4}+$$

$$\frac{1}{x z^4}+\frac{x}{z^4}+\frac{x^3}{z^4}+\frac{x}{y^2 z^4}+\frac{x^2}{y^2 z^4}+\frac{x y}{z^4}+\frac{x^3 y}{z^4}+\frac{1}{z^3}+\frac{x^2}{z^3}+\frac{1}{y z^3}+\frac{x^2}{y z^3}+\frac{1}{z^2}+\frac{x^3}{z^2}+$$

$$\frac{1}{y z^2}+\frac{x^2}{y z^2}+\frac{x y}{z^2}+\frac{x^3 y}{z^2}+\frac{1}{z}+\frac{x^3}{z}+\frac{1}{y z}+\frac{x}{y z}+\frac{x y}{z}+\frac{x^3 y}{z}+x y z+x^2 y z,$$

$$1+x+y+x y+\frac{1}{x^3 y^3 z^7}+\frac{1}{x y^3 z^7}+\frac{1}{x^3 y^2 z^7}+\frac{1}{x^2 y^2 z^7}+\frac{1}{x^2 y z^7}+\frac{1}{x y z^7}+\frac{1}{z^6}+\frac{1}{x z^6}+$$

$$\frac{1}{x^5 y^5 z^6}+\frac{1}{x^3 y^5 z^6}+\frac{1}{x^5 y^4 z^6}+\frac{1}{x^3 y^4 z^6}+\frac{1}{x^2 y^4 z^6}+\frac{1}{x y^4 z^6}+\frac{1}{x^4 y^3 z^6}+\frac{1}{x y^3 z^6}+\frac{1}{y^2 z^6}+$$

$$\frac{1}{x^4 y^2 z^6}+\frac{1}{x^3 y^2 z^6}+\frac{1}{x^2 y^2 z^6}+\frac{1}{x^3 y z^6}+\frac{1}{x^2 y z^6}+\frac{1}{x y z^6}+\frac{1}{x^3 y^4 z^5}+\frac{1}{x^2 y^4 z^5}+\frac{1}{x^4 y^3 z^5}+$$

$$\frac{1}{x^3 y^2 z^5}+\frac{1}{x^2 y^2 z^5}+\frac{1}{y z^5}+\frac{x}{y z^5}+\frac{y}{z^5}+\frac{x y}{z^5}+\frac{1}{z^4}+\frac{1}{x z^4}+\frac{x^2}{z^4}+\frac{1}{x^3 y^3 z^4}+\frac{1}{x^2 y^3 z^4}+\frac{1}{x^3 y^2 z^4}+$$

$$\frac{x}{y^2 z^4}+\frac{x}{y z^4}+\frac{y}{z^4}+\frac{y}{x z^4}+\frac{x y}{z^4}+\frac{x y^2}{z^4}+\frac{x^2 y^2}{z^4}+\frac{1}{z^3}+\frac{1}{x z^3}+\frac{1}{x^2 y^2 z^3}+\frac{y}{z^3}+\frac{y}{x z^3}+\frac{x^2 y}{z^3}+\frac{x y^2}{z^3}+$$

$$\frac{x^2 y^2}{z^3} + \frac{1}{x z^2} + \frac{x}{z^2} + \frac{x^2}{z^2} + \frac{x}{y z^2} + \frac{x y}{z^2} + \frac{x y^2}{z^2} + \frac{x^2 y^2}{z^2} + \frac{1}{z} + \frac{1}{x z} + \frac{x^2}{z} + \frac{1}{y z} + \frac{1}{x y z} + \frac{x y}{z} + \frac{x^2 y}{z},$$

$$x + x^2 + \frac{1}{y} + \frac{1}{x y} + \frac{1}{x^2 y^3 z^7} + \frac{1}{x y^3 z^7} + \frac{1}{x^2 y^2 z^7} + \frac{1}{x y^2 z^7} + \frac{1}{x^4 y^5 z^6} + \frac{1}{x^3 y^5 z^6} + \frac{1}{x^4 y^4 z^6} +$$

$$\frac{1}{x y^4 z^6} + \frac{1}{x^2 y^3 z^6} + \frac{1}{x y^3 z^6} + \frac{1}{y^2 z^6} + \frac{1}{x^3 y^2 z^6} + \frac{1}{x^2 y^2 z^6} + \frac{1}{y z^6} + \frac{1}{x y z^6} + \frac{1}{z^5} + \frac{x}{z^5} + \frac{1}{x^4 y^5 z^5} +$$

$$\frac{1}{x^3 y^5 z^5} + \frac{1}{x^4 y^4 z^5} + \frac{1}{x^2 y^4 z^5} + \frac{1}{x y^4 z^5} + \frac{1}{x^3 y^3 z^5} + \frac{1}{x^2 y^3 z^5} + \frac{1}{y^2 z^5} + \frac{1}{x^3 y^2 z^5} + \frac{1}{x y^2 z^5} +$$

$$\frac{1}{x y z^5} + \frac{x}{y z^5} + \frac{1}{z^4} + \frac{1}{x z^4} + \frac{x^2}{z^4} + \frac{1}{x^2 y^4 z^4} + \frac{1}{x^3 y^3 z^4} + \frac{1}{x^2 y^3 z^4} + \frac{x}{y^2 z^4} + \frac{1}{y z^4} + \frac{x}{y z^4} + \frac{x y}{z^4} +$$

$$\frac{x^2 y}{z^4} + \frac{1}{z^3} + \frac{1}{x z^3} + \frac{x^2}{z^3} + \frac{x}{y^2 z^3} + \frac{1}{y z^3} + \frac{x}{y z^3} + \frac{x y}{z^3} + \frac{x^2 y}{z^3} + \frac{x^2}{z^2} + \frac{x y}{z^2} + \frac{x^2 y}{z^2} + \frac{1}{y z} + \frac{x}{y z} + z + x z,$$

$$x + x^2 + x y + x^3 y + \frac{1}{y^3 z^7} + \frac{1}{x^2 y^3 z^7} + \frac{1}{y^2 z^7} + \frac{1}{x^2 y^2 z^7} + \frac{1}{x^4 y^5 z^6} + \frac{1}{x^2 y^5 z^6} + \frac{1}{y^4 z^6} +$$

$$\frac{1}{x^4 y^4 z^6} + \frac{1}{x^3 y^4 z^6} + \frac{1}{x y^4 z^6} + \frac{1}{x^3 y^2 z^6} + \frac{1}{x^2 y^2 z^6} + \frac{1}{x y^2 z^6} + \frac{x}{y^2 z^6} + \frac{1}{x y z^6} +$$

$$\frac{x}{y z^6} + \frac{1}{z^5} + \frac{x^2}{z^5} + \frac{1}{x^2 y^4 z^5} + \frac{1}{x y^4 z^5} + \frac{1}{x^3 y^3 z^5} + \frac{1}{x y^3 z^5} + \frac{1}{y z^5} + \frac{x^2}{y z^5} + \frac{1}{z^4} +$$

$$\frac{1}{x z^4} + \frac{x}{z^4} + \frac{x^3}{z^4} + \frac{x}{y^2 z^4} + \frac{x^2}{y^2 z^4} + \frac{x y}{z^4} + \frac{x^3 y}{z^4} + \frac{1}{z^3} + \frac{x^2}{z^3} + \frac{1}{y z^3} + \frac{x^2}{y z^3} + \frac{1}{z^2} + \frac{x^3}{z^2} +$$

$$\frac{1}{y z^2} + \frac{x^2}{y z^2} + \frac{x y}{z^2} + \frac{x^3 y}{z^2} + \frac{1}{z} + \frac{x^3}{z} + \frac{1}{y z} + \frac{x}{y z} + \frac{x y}{z} + \frac{x^3 y}{z} + x y z + x^2 y z,$$

$$1 + x + y + x y + \frac{1}{x^3 y^3 z^7} + \frac{1}{x y^3 z^7} + \frac{1}{x^3 y^2 z^7} + \frac{1}{x^2 y^2 z^7} + \frac{1}{x^2 y z^7} + \frac{1}{x y z^7} + \frac{1}{z^6} + \frac{1}{x z^6} +$$

$$\frac{1}{x^5 y^5 z^6} + \frac{1}{x^3 y^5 z^6} + \frac{1}{x^5 y^4 z^6} + \frac{1}{x^3 y^4 z^6} + \frac{1}{x^2 y^4 z^6} + \frac{1}{x y^4 z^6} + \frac{1}{x^4 y^3 z^6} + \frac{1}{x y^3 z^6} + \frac{1}{y^2 z^6} +$$

$$\frac{1}{x^4 y^2 z^6} + \frac{1}{x^3 y^2 z^6} + \frac{1}{x^2 y^2 z^6} + \frac{1}{x^3 y z^6} + \frac{1}{x^2 y z^6} + \frac{1}{x y z^6} + \frac{1}{x^3 y^4 z^5} + \frac{1}{x^2 y^4 z^5} + \frac{1}{x^4 y^3 z^5} +$$

$$\frac{1}{x^3 y^2 z^5} + \frac{1}{x^2 y^2 z^5} + \frac{1}{y z^5} + \frac{x}{y z^5} + \frac{y}{z^5} + \frac{x y}{z^5} + \frac{1}{z^4} + \frac{1}{x z^4} + \frac{x^2}{z^4} + \frac{1}{x^3 y^3 z^4} + \frac{1}{x^2 y^3 z^4} + \frac{1}{x^3 y^2 z^4} +$$

$$\frac{x}{y^2 z^4} + \frac{x}{y z^4} + \frac{y}{z^4} + \frac{y}{x z^4} + \frac{x y}{z^4} + \frac{x y^2}{z^4} + \frac{x^2 y^2}{z^4} + \frac{1}{z^3} + \frac{1}{x z^3} + \frac{1}{x^2 y^2 z^3} + \frac{y}{z^3} + \frac{y}{x z^3} + \frac{x^2 y}{z^3} + \frac{x y^2}{z^3} +$$

$$\frac{x^2 y^2}{z^3} + \frac{1}{x z^2} + \frac{x}{z^2} + \frac{x^2}{z^2} + \frac{x}{y z^2} + \frac{x y}{z^2} + \frac{x y^2}{z^2} + \frac{x^2 y^2}{z^2} + \frac{1}{z} + \frac{1}{x z} + \frac{x^2}{z} + \frac{1}{y z} + \frac{1}{x y z} + \frac{x y}{z} + \frac{x^2 y}{z},$$

$$x + x^2 + \frac{1}{y} + \frac{1}{x y} + \frac{1}{x^2 y^3 z^7} + \frac{1}{x y^3 z^7} + \frac{1}{x^2 y^2 z^7} + \frac{1}{x y^2 z^7} + \frac{1}{x^4 y^5 z^6} + \frac{1}{x^3 y^5 z^6} + \frac{1}{x^4 y^4 z^6} +$$

$$\frac{1}{x y^4 z^6} + \frac{1}{x^2 y^3 z^6} + \frac{1}{x y^3 z^6} + \frac{1}{y^2 z^6} + \frac{1}{x^3 y^2 z^6} + \frac{1}{x^2 y^2 z^6} + \frac{1}{y z^6} + \frac{1}{x y z^6} + \frac{1}{z^5} + \frac{x}{z^5} + \frac{1}{x^4 y^5 z^5} +$$

$$\frac{1}{x^3 y^5 z^5} + \frac{1}{x^4 y^4 z^5} + \frac{1}{x^2 y^4 z^5} + \frac{1}{x y^4 z^5} + \frac{1}{x^3 y^3 z^5} + \frac{1}{x^2 y^3 z^5} + \frac{1}{y^2 z^5} + \frac{1}{x^3 y^2 z^5} + \frac{1}{x y^2 z^5} +$$

$$\frac{1}{x y z^5} + \frac{x}{y z^5} + \frac{1}{z^4} + \frac{1}{x z^4} + \frac{x^2}{z^4} + \frac{1}{x^2 y^4 z^4} + \frac{1}{x^3 y^3 z^4} + \frac{1}{x^2 y^3 z^4} + \frac{x}{y^2 z^4} + \frac{1}{y z^4} + \frac{x}{y z^4} + \frac{x y}{z^4} +$$

$$\frac{x^2 y}{z^4}+\frac{1}{z^3}+\frac{1}{x z^3}+\frac{x^2}{z^3}+\frac{x}{y^2 z^3}+\frac{1}{y z^3}+\frac{x}{y z^3}+\frac{x y}{z^3}+\frac{x^2 y}{z^3}+\frac{x^2}{z^2}+\frac{x y}{z^2}+\frac{x^2 y}{z^2}+\frac{1}{y z}+\frac{x}{y z}+z+x z\Big\},$$

$$\Big\{1+\frac{1}{z},\ \frac{1}{x}+\frac{1}{x z},\ 1+\frac{1}{x y}+\frac{1}{x y z},\ 1+\frac{1}{z},\ \frac{1}{x}+\frac{1}{x z},\ \frac{1}{x y}+\frac{1}{x y z},\ 1,\ y,\ 0,\ 1,\ y,\ 0\Big\},$$

$$\Big\{0,\ 1+\frac{1}{z},\ 1+\frac{1}{y},\ 0,\ 0,\ 0,\ x+\frac{1}{y z},\ 0,\ 0,\ x,\ 0,\ 0\Big\},$$

$$\Big\{1+\frac{1}{z},\ 0,\ 1+\frac{1}{x},\ 0,\ 0,\ 0,\ 0,\ y+\frac{1}{x z},\ 0,\ 0,\ y,\ 0\Big\},$$

$$\Big\{x z^2+x y z^2,\ y z^2+x y z^2,\ 0,\ 0,\ 0,\ 0,\ 0,\ 0,\ z^2+x y z^3,\ 0,\ 0,\ x y z^3\Big\},$$

$$\Big\{x y+x y z,\ 0,\ y z+x y z,\ 1+\frac{1}{z},\ 0,\ 1+\frac{1}{x},\ x y+x^2 y+\frac{1}{z}+\frac{x}{z},\ y+x y+x y^2+\frac{1}{z}+\frac{1}{x z}+\frac{y}{z}+x y^2 z,$$
$$1+x y+\frac{1}{z}+x y z,\ x y+x^2 y+\frac{1}{z}+\frac{x}{z},\ y+x y+x y^2+\frac{1}{z}+\frac{1}{x z}+\frac{y}{z}+x y^2 z,\ 1+x y+\frac{1}{z}+x y z\Big\},$$

$$\Big\{0,\ x y+x y z,\ x z+x y z,\ 0,\ 1+\frac{1}{z},\ 1+\frac{1}{y},\ x^2+\frac{x}{y z}+x^2 y z,\ x+x y+\frac{1}{z}+\frac{1}{y z},$$
$$x+\frac{1}{y}+\frac{1}{y z}+x z,\ x^2+\frac{x}{y z}+x^2 y z,\ x+x y+\frac{1}{z}+\frac{1}{y z},\ x+\frac{1}{y}+\frac{1}{y z}+x z\Big\},$$

$$\Big\{x z+x y z,\ y z+x y z,\ 0,\ 1+\frac{1}{y},\ 1+\frac{1}{x},\ 0,\ x y z+x^2 y z,\ x y z+x y^2 z,$$
$$\frac{1}{x y}+z+x y z,\ x y z+x^2 y z,\ x y z+x y^2 z,\ \frac{1}{x y}+z+x y z\Big\}\Big\};$$

In[22]:= `Dimensions[theQCA]`

Out[22]= {12, 12}

In[23]:= `Det[theQCA] // pmod2`

Out[23]= 1

In[24]:= `symprod[theQCA, theQCA] // pmod2 // MatrixForm`

Out[24]//MatrixForm=

$$\begin{pmatrix}
0&0&0&0&0&0&1&0&0&0&0&0\\
0&0&0&0&0&0&0&1&0&0&0&0\\
0&0&0&0&0&0&0&0&1&0&0&0\\
0&0&0&0&0&0&0&0&0&1&0&0\\
0&0&0&0&0&0&0&0&0&0&1&0\\
0&0&0&0&0&0&0&0&0&0&0&1\\
1&0&0&0&0&0&0&0&0&0&0&0\\
0&1&0&0&0&0&0&0&0&0&0&0\\
0&0&1&0&0&0&0&0&0&0&0&0\\
0&0&0&1&0&0&0&0&0&0&0&0\\
0&0&0&0&1&0&0&0&0&0&0&0\\
0&0&0&0&0&1&0&0&0&0&0&0
\end{pmatrix}$$

theQCA is indeed a symplectic transformation, preserving all commutation relations.

## Time-reversal invariance

In[25]:= `realQ[theQCA]`

Out[25]= {0, 0, 0, 0, 0, 0, 0, 0, 0, 0, 0, 0}

Thus, every X or Z is mapped by theQCA to a Pauli operator with an even number of Y tensor components.

---

# Transforming new terms of the Hamiltonian by theQCA

In[26]:=
```
theQCA.newsigma // pmod2 // MatrixForm
```

Out[26]//MatrixForm=

$$\begin{pmatrix} 0 & 0 & 0 & 0 & 1 & 0 & 0 & 0 \\ 0 & 0 & 0 & 1 & 0 & 0 & 0 & 0 \\ 0 & 0 & x\,y\,z^2 & 0 & 0 & 0 & 0 & 0 \\ 0 & 0 & 0 & 0 & 0 & 0 & 1 & 0 \\ 0 & 0 & 0 & 0 & 0 & 0 & 0 & 1 \\ 0 & 0 & 0 & 0 & 0 & 1 & 0 & 0 \\ 0 & 0 & 0 & 0 & 0 & 0 & 0 & 0 \\ 0 & 0 & 0 & 0 & 0 & 0 & 0 & 0 \\ 0 & 0 & 0 & 0 & 0 & 0 & 0 & 0 \\ 0 & 0 & 0 & 0 & 0 & 0 & 0 & 0 \\ 0 & 0 & 0 & 0 & 0 & 0 & 0 & 0 \\ 0 & 0 & 0 & 0 & 0 & 0 & 0 & 0 \end{pmatrix}$$

This manifestly consists of single-qubit X operators.
